# Supplementary material for: Bidding Games and Efficient Allocations
Source: arXiv:1311.0913 source file (2018-08-10)
Supplement: Supplementary file 2 [file bidding_games.appendix.full.tex]

\section{Existence of PSPE}
\label{apx:PSPE_exist}

Let a \emph{first-price game} be a two-player one-shot game of the following form: each player submits a bid $b_i\in \calB$, and the payoffs $u_1,u_2$ are determined only by the higher bid.
\begin{lemma}
\label{lemma:auction}
Consider any sequence of better-replies in a first-price game. Then after the first time a bidder raises her bid, no bidder ever lowers her bid.
%A first-price game  where $\calB$ is finite has a pure Nash equilibrium. Moreover, any sequence of better-replies must converge. % (i.e., the game has an ordinal potential).
\end{lemma}
\begin{proof}
Recall that tie-breaking is in favor of bidder~1.
%Assume, toward a contradiction, that there is a cycle of improvements. 
Suppose that at some step bidder~1 increases her bid from $(b_1,b_2)$ to $b'_1$. Note that $b'_1\geq b_2$, as otherwise $b_1 < b'_1 \leq b_2$ and $(b_1,b_2);(b'_1,b_2)$ lead to the same outcome (if the first increase is by bidder~2 then $b'_2>b_1$). Any further step of bidder~1 must keep $b'_1\geq b_2$, otherwise we just go back to the outcome of $(b_1,b_2)$ (which is weakly worse for bidder~1). 

Consider the next reply by bidder~2 (after all consecutive steps of bidder~1)---he must also increase his bid to some $b'_2>b'_1\geq b_2$ in order to have any effect. Then bidder~1 must increase again and so on. Thus no bidder ever reduces her bid (after the first increase). % and budgets are bounded, the process must converge to a pure Nash equilibrium.
\end{proof}
In the continuous case Lemma~\ref{lemma:auction} alone does not guarantee the bids converge or that a pure equilibrium exists (even in this simple game), since the bid increments may become infinitesimally small. 

We next show that this scenario is impossible in bidding games, as there is some bounded resolution for the budgets.
 Informally, for games at height $k$ the interval $\calB = [0,1]$ can be divided into $2^k$ ``budget intervals'' of equal size. All budget partitions $(B_1,B_2)$ where $B_1$ belongs in the same budget interval, would lead to the same outcomes. 

For intuition, note that for $k=1$ it only matters if $B_1\geq 0.5$, since then white can force a win. For $k=2$, white can force two wins if $B_1\geq 0.75$, select whether to win in the first or second turn if $B_1\in[0.5,0.75)$, etc. 

 The next lemma states this formally.

\begin{lemma}\label{lemma:intervals}
 Let $G$ be a bidding game, and denote $k=\height(G)$.  Let $\gamma$ be some strategy profile in $G$. There is a strategy profile $\gamma^*$ s.t.  for any $j\in \{0,1,\ldots,2^k-1\}$: (a)  $\gamma^*$ and $\gamma$ yield the same outcome under budget $B_1=j\cdot 2^{-k}$; (b)  $\gamma^*$ yields the same outcome under any budget $B_1\in[j2^{-k},(j+1) 2^{-k})$. Also, $\gamma^*$ is a PSPE if $\gamma$ is. 
\end{lemma} 
\begin{proof}
We show by induction on $k$. Clearly for $k=0$ there is just one budget interval, and no strategies. For intuition, note that for $k=1$ it only matters if $B_1\geq 0.5$, since then white can force a win. For $k=2$, white can force two wins if $B_1\geq 0.75$, select one win if $B_1\in[0.5,0.75)$, etc.

 More generally, assume that the lemma holds for height at most $k-1$. We replace $\gamma$ with $\gamma^*$ in all subtrees of $s$. Now we construct $\gamma^*(s)$. For any $j\in\{0,1,\ldots,2^k\}$, $B_1=j 2^{-k}$, set strategies in $\gamma^*(s,B_1)$ as in $\gamma$. Take some $j\in\{0,1,\ldots,2^k-1\}$ and denote the bids under $j2^{-k}$ by $b_1,b_2$. For $B_1 \in [j2^{-k},(j+1) 2^{-k})$, we denote $\delta = B_1-j2^{-k}$. We prove for the case where white wins in $(s,j2^{-k})$, i.e. that $b_1\geq b_2$, and w.l.o.g. $b_2=\min\{b_1,B_2\}$. The proof for the case where black wins is symmetric. We set $b^*_1 = b_1+\delta$ and $b^*_2 = \min\{b^*_1,B_2\}$.  With budget $j2^{-k}$, the remaining budget was $j2^{-k}-b_1 = (2j)2^{-(k-1)}-b_1$.  With the new budget $B_1$, white still wins, and the remaining budget is $B_1-b_1 = j2^{-k}+\delta - (b_1+ \delta) = j2^{-k}-b_1$. Thus (a) and (b) of the Lemma hold by construction. Also, if $\gamma$ is a PSPE, then by construction (and induction) there are no deviations from $\gamma^*$ at the budget points $j2^{-k}, j\in\{0,1,\ldots,2^k\}$. We need to show that there are no deviations as $\tup{s,B_1}$, $B_1 = j2^{-k}+\delta$ for some $j<2^k$ and $\delta<2^{-k}$.

 Clearly black does not have new deviations in $\tup{s,B_1}$, since any such deviation would also be a deviation in $\tup{s,j2^{-k}}$. Suppose that white has a deviation from $b^*_1$ to $b^*_1+\tau$ ($\tau\neq 0$). If $b^*_2=b^*_1$, then $b_2=b_1$ and white had a similar deviation from $b_1$ to $b_1+\tau$. 

Thus suppose that $b^*_2 = B_2 < b^*_1$, and white deviates by decreasing her bid. If $b'_1<b^*_2=B_2$ (white drops), then after bidding black has $0$ budget. Since $b_2+\delta\geq B_2 = 1-j2^{-k}-\delta$ we have that at $\tup{s,j2^{-k}}$, the remaining budget of black if white drops is $1-j2^{-k}-b_2 \leq 1-j2^{-k} - (1-j2^{-k}-2\delta) = 2\delta < 2^{-(k-1)}$. Thus by induction, the outcome under $\tup{s,j2^{j-1}}$ (with winning bid $b_2$) and under $\tup{s,B_1}$ (with $b^*_2$) is the same: both fall in the budget interval $B'_2\in(0,2^{-(k-1)}]$ (equivalently, $B_1\in [1-2^{-(k-1)},1)$). 

If $b'_1\geq b^*_2$ (white still takes). Then we claim that $B_1-b^*_1,B_1-b'_1$ belong to the same budget interval. Suppose otherwise, then since $|b^*_1-b'_1|<\delta$, $B_1-b^*_1$ is close to the right end of its interval, i.e.,   $j2^{-k}-b_1 = B_1-b^*_1 \in [j'2^{-(k-1)}-\delta, j'2^{-(k-1)})$ for some $j\leq 2^{k-1}$. Rearranging, 
$$b_1 \in (2j2^{-(k-1)} - j'2^{-(k-1)}, 2j2^{-(k-1)} - j'2^{-(k-1)}+\delta] = ((2j-j')2^{-(k-1)}, (2j-j')2^{-(k-1)}+\delta].$$
Thus we have $b_2 \leq b_1 \leq j'' 2^{-(k-1)}+\delta$ for some $j''<2^{k-1}$. This means that 
$$B_1+b_2 +\delta =   2j2^{-(k-1)} + b_2 +\delta \leq j'2^{-(k-1)}+2\delta < (j'+1)2^{-(k-1)} \leq 1,$$
and thus $b_2+\delta \leq 1-B_1 = B_2$. This implies that $b_1=b_2$ (it cannot be that $b_2=B_2$ for $\delta>0$), and thus $b^*_1 = b_1+\delta < B_2$. This is a contradiction to the selection of $b^*_2 = B_2 < b^*_1$ above.
\end{proof}

\begin{rtheorem}{th:PSPE}
Algorithm~\ref{alg:PSPE} computes a PSPE of $G$. 
\end{rtheorem}

\begin{proof}
Let $k=\height(G)$.
Note that the algorithm effectively goes over all states $s\in S\setminus T$ from the bottom up, and for for any possible budget allocation within the given resolution $\eps=2^{-k-2}$, runs an auction where players iteratively modify their bids, until none of them can gain by further modifying her bid.

We prove by induction on the height of the tree. The base case is trivial since in a tree of height $0$, $S\setminus T$ is empty.

We first set the next states players select in $s$.  Let $g(s) = \{s_1,\ldots,s_q\}$. By the induction hypothesis, for each subgame $G|_{s_j}$ our algorithm has computed some PSPE $\gamma|_{s_j}$. Thus in each $s_j$ there is a mapping $\mu_j :\calB \rightarrow T(G)$. 
For every $B^*_i$, let $s^*_i(B^*_i) \in \argmax_{s'\in g(s)}u_i(\mu_j(B^*_i))$, i.e., the best next state for $i$ under remaining budget $B^*_i$.

This defines a first-price game played in state $(s,B_1)$: For every $b_1 \geq b_2$, the outcome is $t^*=\mu_{s^*_1}(B^1-b_1)\in T(G)$, and thus utilities $u_1(t^*),u_2(t^*)$ are only determined by the higher bid $b_1$. Similarly when $b_2>b_1$.  

By Lemma~\ref{lemma:auction}, bids can only increase.  By Lemma~\ref{lemma:intervals}, whenever white increases her bid $b_1$, she can w.l.o.g. set the bid $b'_1$ so that $B_1-b'_1$ is a multiple of $\eps$. Thus there is only a finite number of bid increments, from any initial state.

We further note that if $\mu_j$ is monotone for all $s_j$ (that is, more budget never hurts the player), then the minimal increase in Algorithm~\ref{alg:PSPE} takes a particularly simple form. If a player gains by bidding $b'_i > b_i$, it is always best to increase by the minimal amount that guarantees winning the turn (and leaves the player with maximal remaining budget). Thus all increments are by one unit of $\eps$: The black player always increases to $b'_2 = b_1+\eps$, and the white player always increases to $b'_1 = b_2$. 
%[show (as a lemma?) that we only care if $B_1\in[k 2^h,(k+1)2^h)$]
%
%The only difference is that we are required to prove that the auction at the current step maintains the property of being upward closed for bids of player~2. Fix $b_1$. For every $b_2>b_1$, player~2 can select from $\{s_1,\ldots,s_{k}\}$ (all states in $g_2(s)$, and a particular state in $g_1(s)$), and get a utility of $u^j_2(B_2-b^*)$ for selecting $s_j$. Recall that by our induction hypothesis, the outcome in every subtree $G|_{s_j}$ is upward closed, and denote $u_2(b_1,b_2)=u_2(t(b_1,b_2))$ (see proof of the discrete case). 
%
%It is left to prove that the auction is upward closed. We set $R=2^{height(s)$. 
%Next, consider some $b^*$.
%If $b^*>b_1$, then for a sufficiently small $\eps>0$, we have for every $b_2\in[b^*-\eps,b^*]$ that 
%$$u_2(b_1,b_2) = \max_{j\leq k} u^j_2(B_2-b_2) = \max_{j\leq k} u^j_2(B_2-b^*)  = u_2(b_1,b^*).$$
%If $b^*\leq b_1$, we have the same outcome for any $b_2\leq b^*$ by the rules of the auction.\footnote{Note that this is where we use the consistent tie-breaking in favor of player~1. In the literature of sequential auctions, existence of a PSPE used various workarounds for the tie-breaking problem. See \cite{gale2001sequential,leme2012sequential}.}
\end{proof}

%
%\begin{lemma}
%Algorithm~\ref{alg:PSPE} computes the Lower PSPE of $G$.
%\end{lemma}
%\begin{proof}[Proof that $\gamma$ is a PSPE]
%We prove by induction on the height of the tree. %Let $B_1\in[0,1]$. By the induction hypothesis,  in eah subgame $G_l,G_r$ there is an surjective monotone mapping $\mu_l:[0,1]\rightarrow T_P(G_l),\mu_r:[0,1]\rightarrow T_P(G_r)$. In each of $G_l,G_r$, we fix the PSPEs that implement $\mu_l,\mu_r$.

%PSPE for every budget $B$, that reaches a Pareto efficient outcome.  By monotonicity and since every Pareto outcome is reachable, we can construct an surjective mapping from $[0,1]$ to the sorted set of Pareto outcomes in $G_l$, and implement this mapping in PSPE. Same for $G_r$. Denote by $t_h(B)$ ($h\in\{r,l\}$) the implemented outcome in $G_h$ under budget $B$.

%We first show that $\gamma$, as computed by Algorithm~\ref{alg:PSPE}, is indeed a PSPE.
%Since $\gamma_l,\gamma_r$ are fixed, we have a normal-form game in $s_0$ (as in Lemma~\ref{lemma:auction}). Suppose both players start from $0$ bids. 

\subsection{Genericity and uniqueness}
\label{apx:gen_uniq}
%For a multiset $A$, denote by $uniq(A)$ the set that contains one copy of each element in $A$.
%\begin{definition}[Genericity]
%We say that a game $G$ is \emph{generic} if each player has a total order over outcomes $T(G)$. $G$ is \emph{weakly generic} if each player has a total order over $uniq(T(G))$.
%\end{definition}
%We observe that in a DAG, genericity and weak-genericity are equivalent.
Generic games are games where agents have strict preferences over all outcomes.
In classical extensive-form games (without bidding), it is known that genericity entails the existence of a unique PSPE. %It can be similarly shown that weak genericity entails that all PSPEs reach the same outcome (possibly via different paths) in a DAG. 
However in our game there are  simultaneous steps, and thus genericity may not be sufficient for uniqueness.

\paragraph{Multiple PSPEs}
%\label{sec:unique}
Our next example shows that the Lower PSPE may not be unique, and that there may be other PSPEs that may not have the same properties.

\begin{proposition}
\label{th:two_PSPE}
There is a generic bidding game with PSPEs that lead to different outcomes under the same budget.
\end{proposition}
\input{example_two_PSPEs_b}
\begin{proof}
Consider the game $G_{\two}$ in Fig.~\ref{fig:two_PSPE}, with budgets $(0.5,0.5)$. The first PSPE we describe starts with a bidding of $b_1=b_2=0$ in $s_0$. White wins and remains with budget $0.5$. With this budget she can win one more bidding phase and thus selects $x$. The game ends in terminal $(5,5)$ (marked with $*$) regardless of the bids in $x$, since if the winner in $x$ goes to $y$ he will lose the next round and get $1$. We note that black would bid strictly above $0$, since otherwise white would bid $0$ and still reach $(9,1)$. 

Next, consider a PSPE that starts with bids $b_1=b_2=0.5$. White wins the turn and remains with a budget of $0$. If she selects $x$, then black can play two turns in a row and reach $(1,9)$. Thus white will select terminal $(2,2)$ (marked with $**$).  This is an equilibrium: black clearly cannot change the outcome. If white lowers her bid, then black wins and remains with a budget of $0$. Then from the same consideration he would avoid selecting $x$ (as white would then reach $(9,1)$). Thus white cannot strictly gain by lowering her bid below $0.5$.
\end{proof}

\section{Games with Discrete Budgets}
\label{apx:discrete}

\begin{rproposition}{th:discrete}
For any $k\in \mathbb N$ there is a binary bidding game $G_k$, s.t. if $G_k$ is played with a discrete budget of $M<2^k$, it has no Pareto-optimal PSPE.
\end{rproposition} 

\begin{proof}
If $M$ is small, a Pareto-efficient outcome may not be reachable in equilibrium under certain budget partitions. Consider the binary game $G_k$, described in Figure~\ref{fig:discrete_PSPE}. In order to reach one of the Pareto-optimal leaves (marked with $*$), the same player must win $k$ times in a row. Suppose that the budget is $M<2^k$. In any budget partition except when $B_2=0$, it holds for both players that $2^{k}B_{i} \gtmi B_{-i}$. Since the budget of the loser doubles with each loss, no agent can win in all $k$ times. Thus the game must end in one of the ``side'' leaves, which are Pareto-dominated.
\end{proof}
\input{example_bad_PSPE_discrete}

\subsection{Monotonicity}
While the proposition above shown that with a small discrete budget we cannot guarantee Pareto efficiency, we can still guaranty that the game is monotone in the following sense. 
\begin{definition}[Monotonicity]
\label{def:mon}
A game $G$ is \emph{monotone}, if adding more budget to a player cannot make her worse off. Formally, if for all $B'_i>B_i$,  there is a PSPE that yields under $B'_i$ an outcome that is at least as good for $i$ as \emph{any} PSPE under $B_i$.
\end{definition}

%Denote by $u_i^*(B_i)$ the highest utility that $i$ can achieve under \emph{any} PSPE with budget $B_i$. 
%We say that a game $G$ is \emph{monotone}, if for all $B'_i>B_i$, we have $u^*_i(B'_i) \geq u^*_i(B_i)$.

 Note that if $G$ is monotone, then it has at least one monotone PSPE (say, the one maximizing the utility of player~1 for every budget). However, the existence of a monotone PSPE in $G$ does not entail that $G$ is itself monotone. Thus Theorem~\ref{th:monotone} is not implied by our main result even in the continuous case.

The following theorem is valid for games with either discrete or continuous budgets.  
\begin{theorem} \label{th:monotone}
Any  binary tree game $G$ is monotone.
\end{theorem}

\begin{proof} 
We prove by induction on the height of the game tree. For height $0$ it is obvious. Note that for height $1$ it is also easy, as there will be exactly one auction round, and the player with the higher budget can force her preferred outcome. 

Let $\gamma$ be some PSPE in $\tup{G,B_1,B_2}$, and suppose $B'_1=B_1+\Delta$ for some $\Delta>0$. 
Suppose we are in the discrete model. Then w.l.o.g. it is sufficient to show for $\Delta=1$. Similarly, in the continuous model it is sufficient to show for $\Delta=\eps$, where $\eps<2^{-\height(G)-2}$, since for any $\eps'<\eps$, the game  $\tup{G,B_1+\eps',B_2-\eps'}$ is either equivalent to $\tup{G,B_1,B_2}$ or to $\tup{G,B_1+\eps,B_2-\eps}$. Thus assume $\Delta=\eps$ (where in the discrete case $\eps=1$).

Intuitively, the proof shows that after the increase, either white can increase her winning bid by $\eps$ in order to discard the excessive budget, or she can lower her losing bid by $\eps$. In either case she can keep the same budget after the auction, and reach an outcome that is at least as good.

Denote by $s_l,s_r$ the left and right children of $s_0$, respectively. Each child is the root of another  binary subgame, which we denote by $G_l,G_r$.  Denote by $\gamma_l,\gamma_r$ the derived PSPEs in each subgame. We can assume w.l.o.g. that each of $\mu_l,\mu_r$ yields the highest possible utility for white under any budget. By induction, $G_l$ and $G_r$ are monotone, and thus $\gamma_l,\gamma_r$ are also monotone.\footnote{This follows since if there is some PSPE better for white under a higher budget $B'_1$, the best PSPE for white under $B'_1$ must hold this as well.} 

Case~I:  player~1 takes round $s_0$ in $\gamma$. That is, $b_1\geq b_2$, and player~1 selects the next move. 
%This is the easy case, and proving monotonicity does not require any assumption on the game tree, or even the induction hypothesis. By increasing her bid from $b_1$ to the optimal point $b'_1=b_1+\eps$, white still wins and remains with exactly the same budget as before ($B'_1-b'_1 = B_1-b_1$). The bids $(b'_1,b_2)$ may not be in equilibrium ($b_2$ may not even be valid if $b_2>B'_2$). However in any equilibrium the utility of white is at least the utility of bidding $b'_1$: if the equilibrium bid is lower than  $b'_1$
W.l.o.g. she selects $G_l$, which means that $t^*= \mu_l(B_1-b_1) \succeq_1 \mu_r(B_1-b_1)$. %$u_1(\gamma_l,B_1-b_1) \geq u_1(\gamma_r,B_1-b_1)$. 
Due to monotonicity of both sub-PSPEs, white is always weakly better off by reducing her bid down to the tie point, thus w.l.o.g. $b_1=b_2=b$. 
Since this is a PSPE in $s_0$, white cannot gain by reducing her bid and dropping the round, which either means that black would pick $s_r$ and (weakly) hurt white, or that black would also pick $s_l$ but without changing the utility of white. Thus either $t'_r \equiv \mu_r(B_2-b) \succeq_2 \mu_l(B_2-b)$, %$u_2(\gamma_r,B_2-b) \geq u_2(\gamma_l,B_2-b)$ 
and $t'_r \preceq_1 t^*$; %$u_1(\gamma_r,B_1+b) \leq u_1(\gamma_l,B_1-b)$; 
or $t'_l = \mu_l(B_2-b) \succeq_2 t'_r$, and $t'_l =_1 t^*$. %$u_2(\gamma_r,B_2-b) \leq u_2(\gamma_l,B_2-b)$ and $u_1(a_l,B_1+b) = u_1(a_1,B_1-b)$. 

Case~Ia:  $B'_2 \geq b+\eps$. We increase both bids in $s_0$ by $\eps$, so that $b'_1=b'_2 = b' = b+\eps$. Note that white still takes the round, and selects $G_l$ with the same budget $B'_1-b' = B_1-b$. The only new deviation white has is bidding higher than $B_1$, but this is clearly pointless due to monotonicity of the subgames. Any deviation for black (i.e. bidding $b'_2>b'$) was also possible before by bidding $b_2>b$, thus it cannot be beneficial. Note that in this case 
$$\mu'(B'_1) = \mu'_l(B'_1-b'_1) = \mu_l(B'_1-b'_1) = \mu_l(B_1-b_1)=t^*,$$ % $u_1(\gamma',B'_1) = u_1(\gamma,B_1)=u_1$.
so both players get the same utility as before the budget change.

Case~Ib: $B'_2 < b+\eps$. Since $b+\eps>B'_2+\eps = B_2\geq b$, we have that $B_2=b$, i.e., black cannot increase his bid. We set $b'_1=b'_2=B_2$. We set $b'_1=b_1+\eps$, so that $B'_1-b'_1 = B_1-b_1$. Clearly black cannot deviate, and white can reach the same outcome as before the increase (or maybe to a better outcome with a different bid).

Case~II: white (player~1) drops the first round in $\gamma$ under $B_1$. It is sufficient for black to take the round by $\eps$ (the minimal significant budget unit), so w.l.o.g. $b=b_2 = b_1+\eps$.
 W.l.o.g. black selects $s_r$, which means $t^*=t^*_r\equiv \mu_r(B_2-b_2) \succeq_2 \mu_l(B_2-b_2)$. %$u_2(\gamma_r,B_2-b) \geq u_2(\gamma_l,B_2-b)$. 
This means that white either cannot or does not want to take the round. %Thus either $b>B_1$; or $b\leq B_1$ and $t^* \succeq_1 \mu_l(B_1-b)$. %$u_1(\gamma_l, B_1-b)\leq u_1(\gamma_r, B_1+b)$. 
Now, consider $B'_1 = B_1+\eps$.

Case~IIa: $b_1>0$. In this case both players can reduce their bids so that $b'_2 = b_2-\eps, b'_1=b_1-\eps$. We get that black still wins and $B'_1+b'_2=B_1+b_2$, so that black still selects $s_r$ and reaches $t^*_r$. From here we may have a chain of responses where in each response either white increases her bid and selects $s_l$, or black increases and selects $s_r$ again. If eventually black wins with bid $b''_2\geq b'_2$, then by monotonicity of $\mu_r$, $\mu_r(B'_1+b''_2) \succeq_1 \mu_r(B'_1+b'_2)=t^*_r$. If sequence ends with white wins ($b''_1\geq b''_2\geq b'_2$). Then we have that $t^*=\mu_l(B_1-b''_1) \succ_1 \mu_r(B_1+b''_2) \succeq_1 t^*_r$.

Case~IIb: $b_1=0,b_2=\eps$. In this case white cannot lower her bid. We define $b'_1=b'_2=0$, so that now white wins,and here remaining budget is $B'_1-b'_1 = B_1+\eps = B_1+b_2$. If there is no deviation of black, then clearly the outcome is at as good for white as before, since in particular she can select $s_r$ and reach $\mu_r(B_1-b'_1) = \mu_r(B_1+b_2) = t^*_r$. Assume, towards a contradiction, that black has a deviation.  Such deviation is w.l.o.g. to bid $b''_2=\eps$, select $s_l$. The outcome would be
$$\mu_l(B'_2-b''_2) = \mu_l(B_2-2\eps) \succ_2 \mu_r(B'_2+b'_1) = \mu_r(B_2-\eps) \succeq_2  \mu_l(B_2-\eps),$$
where the last inequality is since black selects $s_r$ with remaining budget $B_2-\eps=B_2-b_2$. Finally,  
$\mu_l(B_2-2\eps)\succ_2 \mu_l(B_2-\eps)$ is a contradiction to the monotonicity of $\mu_l$, so black does not have a deviation. 
\end{proof}
